# Supplementary material for: CAP-VMs: Capability-Based Isolation and Sharing for Microservices
Source: arXiv:2202.05732 source file (2022-06-24)
Supplement: Supplementary file 1 [file 80-appendix.tex]

\section{Appendix}
\appendix

\begin{figure}[h]
\centering
\begin{tikzpicture}
	\begin{axis}[
		legend columns=1,
		legend style={
    			draw=none,
		},
		legend cell align={left},
		legend style={at={(0.75,.10)},anchor=south, font=\scriptsize},
		width  = 1.0\columnwidth,
		height = 6.5cm,
       xmin=2048, xmax=454656,
       ymin=0, ymax=15,
%       style={align=center}, ylabel=$Latency\ (uSec)$,
       xlabel near ticks,
       xlabel={Data size (B)},
       ylabel={Time to copy (msec)},
       ylabel near ticks,
%       ymode=log,
%       xmode=log, 
			     xtick={
61440,
126976,
192512,
258048,
323584,
389120,
454656},
    			  xticklabels={
F000,
1F000,
2F000,
3F000,
4F000,
5F000,
6F000},xtick scale label code/.code={},
     ]
\addplot[
		each nth point={1},
		dash dot, ACMRed,  thick, mark=*,mark options={solid, scale=0.75},
		] table[x =x, y =y]{tlb.txt};
%\addlegendentry{}

	\end{axis}
\end{tikzpicture}

\caption{TLB threshing with memcpy}
\label{fig:tlb}	
\end{figure}
